# Supplementary material for: Improving Self-Supervised Learning by Characterizing Idealized Representations
Source: arXiv:2209.06235 source file (2022-12-12)
Supplement: Supplementary file 1 [file proofs.tex]

First, we will show that the minimal sample size on size to perform all downstream invariant task is at least the number of equivalence classes.
This should not be a surprise as any task that differs only on one equivalent class will also be in $\tasksinv{}$ so one needs to at least see one example per equivalence class to know which is the current task.

\begin{lemma}\label{lemma:min_n_samples}
The required sample size for any discriminative encoder $\p{Z|X} \in \dP{}$ is $\rS{} \geq |\mathcal{X} / \sim|$.
\end{lemma}
\begin{proof}
Suppose that $\rS{} < |\mathcal{X} / \sim|$.
I.e., for any invariant task $Y \in \tasksinv{}$ there exists a dataset $\Dy$ of size $|\Dy| < |\mathcal{X} / \sim|$ s.t. all ERM $\hat{f} \in \eBQ(\Dy)$ is a Bayes predictor $f \in \BQ{}$.
Importantly this means that for any $\Dy$ there is at least one equivalence class $[x]_{miss}$ for which no member of it are in $\Dy$.
As the encoder is discriminative and by \cref{lemma:achieve_0}, we have that for any deterministic function $g$ that is invariant w.r.t. $(\Xc,sim)$ there must exist a function $f \in \Q$ s.t. $f(Z) = g(X)$.
In particular there exists two functions $f,f' \in \Q$ that achieve predict the correct labeling for all representation from coming from examples in $\Dy$ but predict differently on examples coming from the missing equivalence class $[x]_{miss}$.
By construction $f,f' \in \eBQ(\Dy)$ are ERM's but cannot both be actual risk minimizers.
Contradiction.
\end{proof}

\Cref{lemma:min_n_samples} shows that even when the dataset can have different inputs $X$ they need to contain at least one example per equivalence class. 
We now show that this lower bound is achievable by representations that are essentially maximal invariants (or stochastic versions thereof).
Furthermore, any dataset that have at least one single example per equivalence class then ensures that ERM's from these sample efficient encoders are population risk minimizers.

\begin{lemma}[Sample efficient encoders]\label{lemma:sufficient_data}
Let $\p{Z|X} \in \dP{}$ be a discriminative encoder.
Any set $\Sc$ containing an example from each equivalence class is sufficient for $\Q,\tasksinv{},Z$ if the support of the encoder is a maximal invariant, \ie, $\supp{p(Z|x)} = \supp{p(Z|x^+)} \iff x \sim x^+$.
\end{lemma}
\begin{proof}
\begin{itemize}
\item Show that any $D$ with more than an example per equivalence class is redundant, so focus on one per class.
\item Show that for any $D$ with one equivalence per class if you achieve empirical bayes risk you learn how to predict the most likely label perfectly (because discriminative)
\item say that most likely label is a bayes predictor for population task
\item conclude by saying that all empirical bayes predictors predict a population bayes predictor as desired.
\end{itemize}
\end{proof}

Note that when family is unconstrained $\U$ \cref{lemma:sufficient_data} can actually be shown to be an if and only if statement.
For the case of constrained functional essentially any representations s.t. Bayes predictors are cannot distinguish between the support of equivalent examples will be sample efficient. 
As this depends on the task and the Bayes predictors, we only gave the simpler statement of having the same conditional support.

Putting both previous statements together gives directly  \cref{prop:sample_eff_encoder}.

\begin{manualprop}{\ref{prop:sample_eff_encoder}}
Let $\p{Z|X} \in \dP{}$ be a discriminative encoder.
The required sample size is $\rS{} \geq |\mathcal{X} / \sim|$ with equality if  $\supp{p(Z|x)} = \supp{p(Z|x^+)} \iff x \sim x^+$.
\end{manualprop}
\begin{proof}
$\rS{} \geq |\mathcal{X} / \sim|$ due to \cref{lemma:min_n_samples}.
Equality comes from \cref{lemma:sufficient_data}.
\end{proof}

\Cref{prop:sample_eff_support} only concerns the best case dataset (minimal number of samples), but we can easily convert it into a statement about average case dataset (expected number of samples to see) using results from the coupon collector problem.
For simplicity let us only consider tasks that are deterministic labeling of the inputs.
Then expected number of samples (over \iid samples from $\p{X,Y}$) s.t. for any invariant task, all empirical Bayes predictors are population Bayes prediction is simply the expected number of samples before sampling one example per equivalence class.
When the inputs are s.t. that that the equivalence classes are equiprobable.
We know by standard coupon collector results that this expected number scales as $\Theta(|\Xc / \sim| \log |\Xc / \sim|)$, as seen for example in \citet{ross_first_2010}.
In the non-equiprobable case, one can use results from the weighted coupon collector problem.
For example, if the sorted distribution of equivalence class is $\mathbf{p} = (p(M(X)=m_1), \dots, p(M(X)=m_{|\Mc|})$ where $\mathbf{p}_i \leq \mathbf{p}_{i+1}$.
Then the expected number of samples will essentially scale as $\sum_{i=1}^{|\Mc|} \frac{1}{i \cdot \mathbf{p}_i }$ \cite{berenbrink_weighted_2009}.

% \begin{corollary}
% Let $\p{Z|X}$ be an encoder that satisfies the support constraint from \cref{prop:sample_eff_support}.
% Let $X$ and $(\Xc,\sim)$ be s.t. that the probability of each equivalence class is the same, \ie, $p([x]) = p([x'])$ for all $x,x' \in \Xc$.
% Let $Y$
% Then the expected (over sampling from $\p{X,Y}$) number of samples $|\Dy|$ drawn \iid from $\p{X,Y}$ s.t. for any 

% Then the expected (over 

% Let $\Dy$ be a dataset of $\iid$ samples from the joint $\p{X,Y}$
% \end{corollary}

\subsection{Proofs for sample space $\Zc$}

One simple and useful lemma is that considering stochastic encoders does not change the requirements on the sample space.

\begin{lemma}[Deterministic is sufficient]\label{lemma:det_sufficient}
Let $\p{Z|X}$ be an encoder that can be shattered by $\Q$ w.r.t. $(\Xc,\sim)$.
Then there exists a deterministic representation $Z_{det} = e(X)$ that t.v.i. $\Zc_{det} \subseteq \supp{\p{Z}}$ and can be shattered by $\Q$ w.r.t. $(\Xc,\sim)$.
\end{lemma}
\begin{proof}
Suppose that $\p{Z|X}$ is s.t. for any binary labeling $b \in 2^{\Mc}$ there exists $\pred{} \in \Q$ s.t. $f(Z) = b(M(X))$. 
Then one can easily construct a deterministic encoder mapping $x$ to a point in the conditional support, \eg (one of) the mode(s) $e : x \to \argmax_z p(z|X)$,  that would satisfy $f(e(x)) = b(M(X))$.
Clearly the resulting support cannot be larger than the original one and so $\supp{p(Z_{det})} \subseteq \supp{p(Z)}$.
Then let $\Zc_{det} = \supp{p(Z_{det})}$ which concludes the proof.
\end{proof}

First, let us prove that that the the necessity of shattering w.r.t. $\Q,\sim$ is tightly related to the VC dimension of $\Q$.
This should not be surprising given that VC dimension is tightly related to classical shattering, which is itself tightly related to our invariant shattering.

\begin{manualprop}{\ref{prop:VC_dimension}}[Invariant shattering and VC dimension]
There exists a discriminative encoder $\p{Z|X} \in \dP{}$ if and only if the VC dimension of $\Q$ is at least the number of equivalence classes, \ie,  $\op{VC}{\Q} \geq |\mathcal{X} / \sim|$.
\end{manualprop}
\begin{proof}
By \cref{lem:induction}, there exists an encoder that is discriminative $\p{Z|X} \in \dP{}$ if and only if there exists a shattered encoder $\p{Z|X} \in \sP{}$.
Now let us show that shattering if possible if and only if $\op{VC}{\Q} \geq |\mathcal{X} / \sim|$.
As any maximal invariant is a bijection from the quotient set to some $\Mc$, the cardinality of the image of $\Xc$ by $M$ is $|\mathcal{X} / \sim|$.

($\impliedby$) Let $\op{VC}{\Q} \geq |\mathcal{X} / \sim|$, then by definition there exists some set of $|\mathcal{X} / \sim|$ points $\mathcal{D} = \set{z_1,\dots, z_n}$ in $\Zc$ that can be (clasically) shattered by $\Q$.
As $\mathcal{D}$ has cardinality $|\mathcal{X} / \sim|$ there exists a maximal invariant $M(X)$ whose image is $\mathcal{D}$, let $p(Z|X)$ be deterministic with $Z = M(X)$. 
By construction $\mathcal{D}$ can be (clasically) shattered by $\Q$ so for any binary labeling $b \in 2^{\Mc}$ there exists a $\pred{} \in \Q$ s.t. $f(Z) = b(Z)=b(M(X))$, \ie, $p(Z|X)$ can is shattered by $\Q$ w.r.t. $(\mathcal{X},\sim)$.

($\implies$) By definition VC dimension is the maximal number of points that can be classically shattered by $\Q$. 
So we know that $\op{VC}{\Q} \geq |\mathcal{X} / \sim|$ implies that there exists no deterministic encoder $Z = e(X)$ s.t. for any binary labeling $b$ there is an $f \in Q$ s.t. $f(e(x)) = b(M(X))$.
Then by \cref{lemma:det_sufficient} we know that there exists also no stochastic encoder  $\p{Z|X}$ s.t. $f(Z) = b(M(X))$. 
\end{proof}

\Cref{prop:VC_dimension} gives the requirement of shattering in terms of VC dimension of $\Q$.
We can thus use all the well known results of VC dimensions to to describe minimal sufficient requirements for shatterability.

\begin{manualcor}{\ref{corr:dimension}}[Dimensionality]
Let $\Zc = \mathbb{R}^{d}$. The minimal and sufficient dimensionality $d_{\Q}$ is the smallest $d$ s.t. there exists a discriminative encoder $\p{Z|X} \dP{}$.
$d_{\Q}$ is:
\begin{itemize}
\item is $d_{\Q_l} = |\mathcal{X} / \sim| - 1$ for linear predictors $\Q_l$;
\item is larger for smaller VC dimensions , \ie,  $\op{VC}{\Q^-}  \leq \op{VC}{\Q} \  \implies  d_{\Q^-} \geq d_{\Q}$;
\item increases for any $\Q^- \subseteq \Q$, \ie,  $  d_{\Q^-} \geq d_{\Q}$;
\item decreases with the number of layers $L$ and hidden neurons per layer $H$ for practical MLPs with ReLU activations $\Q_{LH}$, \ie,  $L^+ \geq L$ and $H^+ \geq H$ $\implies d_{\Q_{L^+H^+}} \leq d_{\Q_{LH}}$;
\item is $d_{\U} = 1$ for universal predictors $\U$.
\end{itemize}
\end{manualcor}
\begin{proof}$ $\\
\begin{itemize}
\item The VC dimension $\Q_l$ with domain $\Zc \subseteq \mathbb{R}^d$ is $d +1$ \cite{shalev-shwartz_understanding_2014}. So by \cref{prop:VC_dimension} we have $d + 1 = \op{VC}{\Q_l} \geq |\mathcal{X} / \sim|$ . And thus $d_{\Q_l} = |\mathcal{X} / \sim| - 1$.
\item Increasing the dimensionality of $\Zc$ from $d^-$ to $d > d^-$ can only increase the VC dimension of $\op{VC}{\Q}$ because $\mathbb{R}^{d^-}$ is (isomorphic to) a subspace of $\mathbb{R}^{d}$. So $\op{VC}{\Q^-}  \leq \op{VC}{\Q} \  \implies  d_{\Q^-} \geq d_{\Q}$.
\item If $\Q^- \subseteq \Q$ then clearly $\op{VC}{\Q^-} \leq \op{VC}{\Q}$. 
So by the previous point we have $d_{\Q^-} \geq d_{\Q}$ as desired.
\item Let $\Q_{LW}$ be an MLP with ReLU activation, $W$ parameters (weight and biases), and $L$ layers. In the practical case of $L \ll W^{0.99}$ we have $\op{VC}{\Q} \in \Theta(WL \log(W))$ \cite{bartlett_nearly-tight_2017}.
In particular the VC dimension increases with $L$ and $W$ and so 
$L^+ \geq L$ and $W^+ \geq W$ $\implies d_{\Q_{L^+W^+}} \leq d_{\Q_{LH}}$.
As the number of weights is proportional to the number of hidden units per layer (and the number of layers) we have $d_{\Q_{L^+H^+}} \leq d_{\Q_{LH}}$ as desired.
\item The VC dimension of $\U$ is clearly infinite even with $d_{\U}$. 
In particular, any set of cardinality $|\Xc / \sim|$ (which is finite due to \cref{assmp:finite_rv}) can be shattered because $|\mathbb{R}| > |\Xc / \sim|$.
\end{itemize}
\end{proof}

\Cref{corr:dimension} only discusses the required dimensionality of $\Zc$, but there is also a cardinality requirement.
Indeed, clearly $Z$ has to take enough possible values to be shatterable $\Zc \geq |\Xc / \sim|$.

\begin{proposition}[Marginal support]\label{prop:marginal_supp}
The minimal sufficient cardinality of the marginal support $\supp{\p{Z}}$ is $|\Xc / \sim|$. I.e.:
\begin{itemize}
\item there exists an encoder $\p{Z|X}$ s.t. $\supp{\p{Z}} = |\Xc / \sim|$ and is discriminative $\p{Z|X} \in \dP{}$;
\item there exists no encoder $\p{Z|X}$ s.t. $\supp{\p{Z}} < |\Xc / \sim|$ and is discriminative $\p{Z|X} \in \dP{}$.
\end{itemize}
\end{proposition}
\begin{proof}$ $\\
(Existence) Take the example from \cref{lem:achieve_0} where $Z$ is a maximal invariant and thus has support $|\Xc / \sim|$.

(Non existence) Suppose that there exists a $\p{Z|X}$ s.t. $\supp{\p{Z}} < |\Xc / \sim|$ and can be shattered $\p{Z|X} \in \sP{}$.
Then by \cref{lemma:det_sufficient} there exists a deterministic encoder $e$ with $\Zc < |\Xc / \sim|$ and can be shattered.
Then by \cref{lemma:disc_shatter} $e$ can be shattered.
As $\Zc < |\Xc / \sim|$ there exists two non equivalent examples $x \not \sim x^-$ s.t. $e(x) = e(x^-)$.
Take any binary labeling $b$ that gives a different label for $[x]$ and $[x^-]$. Then by construction $b(M(x)) \neq b(M(x)^-)$ but $e(x) = e(x^-)$ so there exists no $f$ s.t. $f(Z) = f(e(X)) = b(M(X))$ so $Z = e(X)$ cannot be shattered. Contradiction.
\end{proof}

Note that \cref{prop:sample_space} concerns the minimal and sufficient cardinality of the support $\supp{\p{Z}}$, but this directly implies a minimal and sufficient cardinality of the sample space $\Zc$.

\begin{corollary}[Sample space]\label{cor:sample_space}
The minimal sufficient cardinality of the sample space $\Zc$ is $|\Xc / \sim|$
\end{corollary}
\begin{proof}
This directly comes from \cref{prop:marginal_supp} and letting $\Zc = \supp{\p{Z}}$.
\end{proof}

\subsection{Proofs for augmentations}

\begin{manualprop}{\ref{thm:sufficient_refine}}[Refinement and discriminativeness]
Let $\tasksinv{},M,\Q$ be as in \cref{thm:main}. 
Let $\sim_r \subseteq \sim$ be a refinement of the desired equivalence  with maximal invariant $\Mx{r}$.
Let $\oP{\sim}{M} \defeq \argmin_{p(Z|X) \in \sP{}  } \RiskA{M(X)}{\rv Z}$ denote the encoders that can predict $M$ and are shattered w.r.t $(\mathcal{X},\sim)$.
We have:
\begin{equation} \label{eq:sufficient_refine}
\oP{\sim_r}{\Mx{r}} \subseteq \oP{\sim}{\Mx{r}}  \subseteq \oP{\sim}{M}.
\end{equation}
\end{manualprop}
\begin{proof} $ $\\
($\oP{\sim_r}{\Mx{r}} \subseteq \oP{\sim}{\Mx{r}}$)
By \cref{lemma:near_theorem} we know that any $\p{X|X} \in \oP{\sim}{\Mx{r}}$ achieves $\min \RiskA{M(X)}{Z}$.
So we simply need to show that any $\sPr{} \subseteq \sP{}$.
By definition of a refinement and maximal invariant we know that $x \sim_r x^+ \implies  x \sim x^+ \iff M(x) = M(x^+)$, so $M$ is invariant w.r.t $\sim_r$.
By \cref{lemma:invariant} we thus know that there exists an $h$ s.t. $h \circ \Mx{r} = M$.
Now assume that an encoder $p^r(Z|X) \in \oP{\sim}{\Mx{r}}$ and let $b \in 2^{\Mc}$ be any binary labeling.
Then $b(M(X)) = b(h(\Mx{r}(X)))$.
As $b \circ h \in 2^{\Mc^{r}}$ is a binary labeling for the refinement we must have that there exists $\pred{} \in \Q$ s.t. $f(Z) = b(h(\Mx{r}(X)))$ and so $p^r(Z|X) \in \oP{\sim}{M}$ as desired.

($\oP{\sim}{\Mx{r}}  \subseteq \oP{\sim}{M}$)
From \cref{lemma:induction} and the proof of \cref{lemma:near_theorem} we know that  $\sP{} = \oP{\sim}{M}$ so $\oP{\sim}{\Mx{r}}  \subseteq \oP{\sim}{M}$. Note that it is not equal as encoders in $\oP{\sim}{\Mx{r}}$ have the additional constraint of having to be able to predict $\Mx{r}$ which is not implied by shatterability w.r.t. $\sim$.

\end{proof}

% \begin{proposition}\label{prop:finer_harder_optim}
% Let $p(\A|X)$ and $p(\A'|X)$ be sufficient augmenters.
% If the kernel $\sim_{\A}$ of the Bayes predictor for $\A$ is a refinement of $\sim_{\A'}$, then the resulting encoders satisfy
% \begin{equation}
% \argmin_{p(Z|X) \in \sP{}} \RiskA{\A}{Z} \subseteq 
% \argmin_{p(Z|X) \in \sP{}} \RiskA{\A'}{Z}.
% \end{equation}
% %
% \end{proposition}
% \begin{proof}

% \end{proof}

\subsection{Proofs for functional family}

\begin{proposition}\label{prop:smaller_Q_is_better}
Let $\Qm,\Q$ be families s.t. $\Qm \subseteq \Q$. 
Any $p(Z|X)$ satisfying \cref{thm:main} for $\Qm$ also satisfies it for $\Q$.
\end{proposition}
\begin{proof}
\begin{itemize}
    \item by \cref{lemma:disc_shatter} you only need to show that shattering by smaller functional family is shattering by larger
    \item as $\Qm \subset \Q$ if there exists an $f \in \Qm$ s.t. $f(Z) = b(M(X))$ then there also exists an $f' \in \Qm$ by setting $f' = f$.
\end{itemize}
\end{proof}

\subsection{Proofs for generative models}

In \cref{thm:main} we have seen that to have a discriminative encoder one needs to minimize $\RiskA{M(X)}{Z}$, \ie, be able to classify the index of the equivalence class using the right functional family.
There are three issues for optimizing $\RiskA{M(X)}{Z}$ in practice:
\begin{itemize}
\item we do not have access to a maximal invariant $M(X)$, instead, the invariance structure is given by the ability to sample augmented version of the input $A \dsim p(A|X)$ that retain the invariance structure. As we will show in the following one can instead optimize $\RiskA{A}{Z}$.
\item the second issue comes from the fact that $A$ will likely not take value in $\Mc$. As a result minimizing $\RiskA{A}{Z}$ is ill defined because the loss is not defined on the right space. 
Specifically, $\ell : A,f(Z) \mapsto \indeq{A}{\argmax_m f(Z)[m]}$ will never be equal to 1 as $\argmax_m f(Z)[m]$ will give an integer in $[|\Mc|]$ but $A$ can t.v.i. an arbitrary $\Ac$, \eg, image space.
\item the third issue is that accuracy is not smooth, and in practice we would thus prefer minimizing smooth approximations of it to improve optimization.
\end{itemize}

We will now show that we can solve the three issues by instead minimizing the following Bayes risk $\Risk{A}{Z}$ with respect to most practical losses $\ell$.
Specifically, any information preserving loss.

\begin{definition}[Bayes risk for classification]\label{def:bayes_clf}
Let $\ell : \Ac \times \actspace{} \to \mathbb{R}_{\geq 0}$ be an information preserving loss.
Let $\U \defeq \actspace{}^{[|\Mc|]}$ be the unconstrained predictive family from labels $1, \dots,|\Mc|$ to the action space $\actspace{}$.
The Bayes risk from $Z$ to $A$ w.r.t. $\ell,\Q$ for classification, denoted $\RiskL{A}{Z}{\mathrm{clf},\ell}$, is the Bayes risk when first performing classification and then considering the unconstrained Bayes risk from the predicted class to $A$. I.e. 
\begin{equation}
\RiskL{A}{Z}{\mathrm{clf},\ell} \defeq \inf_{g \in \U} \inf_{f \in \Q} \Ep{\p{A|X}\p{Z|X}}{\ell(A, g(\argmax_m f(Z)[m] )}
\end{equation}
As all Bayes risk w.r.t. $\ell$ are for classification we will simply denote it $\Risk{A}{Z}$.
\end{definition}

It turns out that minimizing the Bayes risk for classification \cref{def:bayes_clf} is equivalent to predicting $M(X)$ when the augmentations $A$ retain the same equivalence structure. 

\begin{proposition}[Using augmentations and losses]\label{prop:using_aug_loss}
Let $\ell$ be any information preserving loss.
Let $\p{A|X}$ be any augmentor s.t. any Bayes predictor $\bayes{A|X}$ is a maximal invariant, \ie, $x \sim x^+ \iff \bayes{A|X}(x) = \bayes{A|X}(x^+)$.
Then:
\begin{equation}
\argmin_{\p{Z|X} \in \sP{}} \RiskA{M(X)}{Z} = \argmin_{\p{Z|X} \in \sP{}} \RiskL{A}{Z}{\mathrm{clf},\ell}  
\end{equation}
\end{proposition}
\begin{proof}$ $\\
First we will show that $\min_{\p{Z|X}} \RiskL{A}{Z}{\mathrm{clf},\ell} =  \Risk{A}{X}$.
Then that an encoder $\p{Z^*|X}$ achieves that risk if and only if $\exists f \in Q$ s.t. $M(X) = \argmax_m f(Z^*)[m]$, which is equivalent to $\p{Z^*|X} \in \argmin_{\p{Z|X}} \RiskA{M(X)}{Z}$.
Finally we note that due to \cref{lemma:achieve_0,lemma:disc_shatter} we have $\argmin_{\p{Z|X}} \RiskA{M(X)}{Z}  = \argmin_{\p{Z|X} \in \dP{}} \RiskA{M(X)}{Z} = \argmin_{\p{Z|X} \in \sP{}} \RiskA{M(X)}{Z}$ and so proving the unconstrained $\argmin_{\p{Z|X}} \RiskA{M(X)}{Z} = \argmin_{\p{Z|X}} \RiskL{A}{Z}{\mathrm{clf},\ell} $ is sufficient.

%Second note that $\p{Z^*|X} \in \argmin_{\p{Z|X}} \RiskL{A}{Z}{\mathrm{clf},\ell}$ if and only if there exists a function $\phi$ s.t. $\phi(Z^*)= M(X)$.,

Let $Z^*$ be the one hot encoding of $M(X)$ as in \cref{lemma:achieve_0} then by letting $f$ be the identity function we have
\begin{align}
\RiskL{A}{Z^*}{\mathrm{clf},\ell} 
&\defeq \inf_{g \in \U} \inf_{f \in \Q} \Ep{\p{A|X}\p{Z|X}}{\ell(A, g(\argmax_m f(Z)[m] )} \label{eq:g_arg_f} \\
&\geq \inf_{g \in \U} \Ep{\p{A|X}\p{Z|X}}{\ell(A, g(M(X))}  & \text{Identity} \\
%&\defeq \RiskQ{A}{M(X)}{\U} \\
&\geq  \Ep{\p{A|X}\p{Z|X}}{\ell(A, \bayes{A|X}(X)}  & \text{\cref{lemma:max_invariant}} \\
&\defeq \RiskQ{A}{X}{\U}
\end{align}
Where we fixed $f$ to be the identity (possible by \cref{assmp:binary_linear}).
We also let $g$ be the function from $M(X)$ to $\bayes{A|X}$ which exists as $\U$ is unconstrained and $\bayes{A|X}$ is a maximal invariant by assumption so there exists a bijection $b$ s.t. $\bayes{A|X} = b(M(X))$.
We thus have $\RiskL{A}{Z^*}{\mathrm{clf},\ell} \geq \Risk{A}{M(X)} \geq \Risk{A}{X}$.
Note that by the risk DPI (\cref{lemma:dpi}) we also have $\RiskL{A}{Z^*}{\mathrm{clf},\ell} \leq \Risk{A}{X}$ from which we conclude $\min_{\p{Z|X}} \RiskL{A}{Z}{\mathrm{clf},\ell} =  \Risk{A}{X}$.

In \cref{eq:g_arg_f} we see that the function mapping $Z$ to $\actspace{}$is a composition between the argmax predictor $\Tilde{f} : Z \to [|\Mc|]$ and the unconstrained $g : [|\Mc|] \to \actspace{}$.
As $\min_{\p{Z|X}} \RiskL{A}{Z}{\mathrm{clf},\ell} = \Risk{A}{X}$ we have that $\Tilde{f} \circ g$ must be equal to a maximal invariant as it must be a equal to a Bayes predictor which by assumption is a maximal invariant.
As $g$'s domain has cardinality $|\Xc / \sim|$ and its image is a maximal invariant, it must be a bijection so by \cref{lemma:max_invariant} $\Tilde{f}$ must also be a maximal invariant.
From which we conclude that $\exists f \in Q$ s.t. $M(X) = \argmax_m f(Z)[m]$.

Now let us show that that $\p{Z^*|X} \in \argmin_{\p{Z|X}} \RiskA{M(X)}{Z}$ if and only if there exists a function $f \in Q$ s.t. $\argmax_m f(Z^*)[m] = M(X)$.
Indeed $\min_{\p{Z|X}} \RiskA{M(X)}{Z} \geq \RiskA{M(X)}{X} = 0$ because $Z=X$ is a valid representation, so we have $\RiskA{M(X)}{Z^*} = 0$ which is achieved if and only if $\exists f \in Q$ s.t. $M(X) = \argmax_m f(Z^*)[m]$ as desired.
\end{proof}

\Cref{prop:using_aug_loss} is very nice as it says that we do not need access to the maximal invariant as long as we have access to the right augmentation.
For example in the case of generative model, it is typical to use the mean squared error, in which case the Bayes predictor is the conditional expectation $\Ep{A}{X}$, the requirement is thus to have $\Ep{A}{X} = \Ep{A}{M(X)}$. 
This will rarely be the case in practice for standard augmentations but by \cref{prop:sufficient_refine} we know that $x \sim x^+ \implies \bayes{A|X}(x) = \bayes{A|X}(x^+)$ is also sufficient, which typically holds in practice. 
E.g. for MNIST it says that the expected (over augmentation) digit should essentially not be another digit.

\subsection{Proofs for contrastive models}

\subsection{Proofs for self-distillation }

\clearpage
\newpage
