# Supplementary material for: Improving Self-Supervised Learning by Characterizing Idealized Representations
Source: arXiv:2209.06235 source file (2022-12-12)
Supplement: Supplementary file 2 [file discriminative.tex]

% Intuitively, the proof of the main theorem goes as follows:
% \begin{enumerate}
%     \item There exists
%     \item \dots
% \end{enumerate}

\ydnote{should add a few bullet points to give the intuition of the proof of main theorem}

First let us show that we can achieve the minimal worst case risk, and let us provide an example of optimal representation.

\begin{lemma}[Perfect worst risk]\label{lemma:achieve_0}
For any $\Q$ that is at least linear with binary weights (\cref{assmp:binary_linear}) there exists an encoder $\p{Z^* | X}$ that achieves the unconstrained worst excess Bayes risk on all $(\Xc,\sim)$-invariant tasks, \ie,
%, \ie, for all $Y \in \tasksinv{}$ we have
\begin{equation}
%\Risk{Y}{Z} = \RiskQ{Y}{Z}{\U}
\min_{\p{Z|X}} \dists{} = 0
\end{equation}
\end{lemma}
\begin{proof}
This can easily be seen by taking $Z^*$ to be a one hot representation of the equivalence class and $\pred{} \in \Q$ be the necessary aggregation function represented as linear equation with binary weights.

Specifically, let $Z^* = \onehot{\nequiv}{M(X)}$ where $M$ is a maximal invariant that maps inputs to an index of the equivalence classes.
Such representation exists by \cref{assmp:rep_space}.

As $\mathbf{e}_i$ is a bijection we have that $Z^*$ is a maximal invariant for $\sim$ by \cref{lemma:max_invariant} because it is a composition between a bijection and a maximal invariant.
By \cref{def:inv_task}, we have that for any $Y \in \tasksinv{}$ the Bayes predictor $\Bpred{}$ is invariant w.r.t. $(\Xc,\sim)$.
As $Z^*$ is a maximal invariant and $\Bpred{}$ is invariant, by \cref{lemma:invariant} there must exist a function $h$ s.t. $h(Z^*) = \Bpred{}(X)$.
\ydnote{need to change to a bayes predictor now (because not all are invariant)}
As the codomain of the Bayes predictor $\Bpred{}$ is also a one hot encoding, we have that $h$ is a function between one hot encodings and can thus be represented by a linear function with binary weights, \ie, $h(Z^*) = W^T Z^*$ where $W \in \set{0,1}^{|\Mc| \times |\Yc|}$ serves as an OR gate.
As $h$ is linear with binary weights it is by \cref{assmp:binary_linear} in $\Q$.
Putting all together we have that for any $Y \in \tasksinv{}$ there exists an $h \in \Q$ so that $\Risk{Y}{Z} \leq \RiskQ{Y}{Z^*}{\set{h}} = \RiskQ{Y}{X}{\set{\Bpred{}}} = \RiskQ{Y}{X}{\U}$.
We conclude the proof by noting that for any $Z$ we have $\Risk{Y}{Z} \geq \RiskQ{Y}{Z}{\U} \geq \RiskQ{Y}{X}{\U}$ where the last inequality comes from the DPI of Bayes risk \cref{lemma:dpi}.
We thus have $\Risk{Y}{Z} = \RiskQ{Y}{X}{\U}$ and so $\dists{} = 0$.
\end{proof}

One important implication of \cref{lemma:achieve_0} is that the set of encoders that are discriminative for the worst-case excess risk is the same as the set of encoders that are discriminative for the average case.
In other words we could replace the supremum in \cref{def:discriminative} by any expectation with support over all invariant tasks, and that would not change any of the theory.

Now we will show that under \cref{assmp:closed}, the binary $\sim$-shatterability from \cref{def:shatter} 
implies $k$-ary shatterability.
The main idea intuition is that we can always achieve predict a desired $k$-ary invariant labelling by combining (due to \cref{assmp:closed}) a ${(k-1)}$-ary predictor with the binary predictor that distinguishes the wrong predictions from the rest.

As previously stated, one can drop \cref{assmp:closed} by changing the binary shatterability requirement to a $k$-ary shatterability (instead of probing it from assumptions).

\begin{lemma}[Binary shatterability implies $k$-ary shatterability]\label{lemma:kary_shatterability}
Let $\Q$ satisfy \cref{assmp:closed}.
If an encoder $\p{Z |X}$ is binary  $(\Xc,\sim)$-shattered by $\Q$ then it is $k$-ary $(\Xc,\sim)$-shattered by $\Q$.
\end{lemma}
\begin{proof}
We will prove the statement by induction, \ie, we suppose that for any $1 < i < k$ we have that $i$-ary shatterability holds and want to prove that it implies $k$-ary shatterability.

We will prove the induction by contradiction. 
Suppose that $k$-ary shatterability does not hold.
Then by definition there exists a $k$-ary invariant labelling $\labelingk{k}$ s.t. no $f_{\scriptscriptstyle k} \in Q$ satisfies $\prediction(f_{\scriptscriptstyle k}(Z)) \aseq \labelingk{k}(X)$. 
Construct $\labelingk{k-1}$ by merging the two last classes, \ie, $\labelingk{k-1}(x) = \labelingk{k}(x)$ if $\labelingk{k}(x) < k $ and $\labelingk{k-1}(x) = k - 1$ otherwise.
By construction $\labelingk{k-1}$ is a ${(k-1)}$-ary invariant labelling so by the induction assumption there exists an $f_{\scriptscriptstyle k-1} \in \Q$ s.t. $\prediction(f_{\scriptscriptstyle k-1}(Z)) \aseq \labelingk{k-1}(X)$.
Now let $\labelingk{2},\labelingk{2}'$ be functions that indicates whether the unpredictable labelling is equal to the last class $\labelingk{2} : x \mapsto \indeq{\labelingk{k}(x)}{k}$ and similarly $\labelingk{2}' : x \mapsto \indneq{\labelingk{k}(x)}{k}$.
By construction $\labelingk{2},\labelingk{2}'$ are binary invariant labelling, so again by the induction assumption there exists an $f_{\scriptscriptstyle 2},f_{\scriptscriptstyle 2}' \in \Q$ s.t. $\prediction(f_{\scriptscriptstyle 2}(Z)) \aseq \labelingk{2}(X)$ and $\prediction(f_{\scriptscriptstyle 2}'(Z)) \aseq \labelingk{2}'(X)$.

By \cref{assmp:closed} we can then use $f_{\scriptscriptstyle k-1},f_{\scriptscriptstyle 2},f_{\scriptscriptstyle 2}'$ to construct the desired an $f_{\scriptscriptstyle k} \in Q$ satisfying $\prediction(f_{\scriptscriptstyle k}(Z)) \aseq \labelingk{k}(X)$.
Specifically, we can construct the function mapping to the logits of class $k-1$ by $f_{\scriptscriptstyle k}^{k-1} = f_{\scriptscriptstyle k-1}(\cdot)[k-1] + f_{\scriptscriptstyle 2}'$, the function mapping to the logits of class $k$ by $f_{\scriptscriptstyle k}^{k} = f_{\scriptscriptstyle k-1}(\cdot)[k-1] + f_{\scriptscriptstyle 2}$ and then concatenate all the logits to get the desired $f_{\scriptscriptstyle k} = \cat{f_{\scriptscriptstyle k-1}(\cdot)[\slice{}k-2]}{f_{\scriptscriptstyle k}^{k-1},f_{\scriptscriptstyle k}^{k}}$.
Indeed, by construction the first $k-2$ classes were already dealt with correctly, and we simply used $f_{\scriptscriptstyle 2}$ and $f_{\scriptscriptstyle 2}'$ a positive component to the right class (we used two functions $f_{\scriptscriptstyle 2},f_{\scriptscriptstyle 2}'$ to deal with zero values logits) and distinguish examples form class $k$ and $k-1$.
The resulting function thus satisfies $\prediction(f_{\scriptscriptstyle k}(Z)) \aseq \labelingk{k}(X)$ which leads to a contradiction.
We thus have that $k$-ary shatterability, which concludes the proof due to induction (the base case being binary).
\end{proof}

% \begin{lemma}[Induction]\label{lemma:induction}
% Let $\Q$ a predictive family satisfying \cref{assmp:binary_linear}.
% If for any $(\Xc,\sim)$-invariant binary labeling $b \in  \set{0,1}^{\Xc}$ there exists an $\pred{} \in \Q$ s.t. $\pred{}(Z) = b(X)$ then for any $(\Xc,\sim)$-invariant $k$-labelling $L \in  \set{1, \dots, k}^{\Xc}$ there exists an $\pred{}' \in \Q$ s.t. $\pred'(Z) = L(X)$.
% \end{lemma}
% \begin{proof}
% \begin{itemize}
% \item use proof by induction to show that if you can predict any invariant $n$-labeling and any binary labeling then you can perform any $(n+1)$-labelling
% \item for any invariant $(n+1)$-labelling $L^+$ you can merge two labels to get an invariant $n$-labelling $L$, which is predictable by assumption of the induction.
% \item now take one of the two labels you merged and perform a one-vs-rest task which is invariant binary labeling
% \item as $\Q$ is closed under compostion of linear functions with binary weight matrices you can sum the result of both preditive tasks
% \item after some algebra easy to show that this will perfectly predict the desired $(n+1)$-labelling.
% \end{itemize}
% \end{proof}

Putting all together let us prove the minimal and sufficient requirement for discriminativeness.

\begin{manualthm}{\ref{thm:main}}[Minimal sufficient requirements for discriminativeness]
Let $M(X)$ be any maximal invariant \wrt{} $(\Xc,\sim)$, and $\tasksinv{}$ be all invariant tasks \wrt{} $(\Xc,\sim)$.
An encoder $\p{Z|X}$ is discriminative for $\tasksinv{},\Q$ if and only if it minimizes the $\Q$-predictability of the maximal invariant while being $(\Xc,\sim)$-shattered by $\Q$, \ie, 
\begin{equation}\label{appx:eq:thm}
\p{Z|X} \in \dP{} \iff \p{Z|X} \in \argmin_{\p{Z|X} \in \sP{}} \Risk{M(X)}{Z}
\end{equation}
\end{manualthm}
\begin{proof}
We will first prove necessity, which comes from the fact that $M(X)$ and binary labeling are in $\tasksinv{}$.
We then prove sufficiency which comes from the fact that by \cref{lemma:kary_shatterability} any invariant labeling can be predicted under shatterability, including predicting all the Bayes predictions.

$(\implies)$ By \cref{lemma:achieve_0}, all discriminative encoders achieve $\Risk{Y}{Z} = \RiskQ{Y}{X}{\U}$ for all $Y \in \tasksinv{}$.
By \cref{def:shatter} any binary invariant labeling $\labelingk{2}$ is an invariant task  $\labelingk{2}(X) \in \tasksinv{}$ as the Bayes predictor $\prediction(\Bpred)=\labelingk{2}$ is invariant.
As $\labelingk{2}(X)$ is a deterministic labeling we have $\Risk{\labelingk{2}(X)}{Z} = \RiskQ{\labelingk{2}(X)}{X}{\U} = 0$. By the definition and non-negativity of the \acc{} loss, there must exist an $f \in \Q$ s.t. $\prediction(f(Z)) \aseq{} \labeling{}(X)$.
As this is true for binary labeling, we have that discriminativeness implies shatterability.
By the same argument we have that maximal invariants are a deterministic invariant task  $M(X) \in \tasksinv{}$, so $\Risk{M(X)}{Z} = \RiskQ{M(X)}{X}{\U} = 0$.
Discriminativness thus implies perfect predictability of maximal invariants, which can be rewritten as a constrained optimizatin problem. 
Indeed, the constrain does not impact the predictability of the maximal invaraint due to the existence of a perfect encoder (\cref{lemma:achieve_0}).
This concludes the necessity proof.

$(\impliedby)$  Suppose that $\p{Z|X}$ is a minimizer of the r.h.s. of \cref{appx:eq:thm}.
By \label{def:inv_task} for any $Y \in \tasksinv{}$ there exists an invariant Bayes predictor $\Bpred$.
As it is an invariant (deterministic) function of $X$, we have that $\prediction(\Bpred(\cdot))$  is also an invariant determinsitic function of $X$ (it is easy to show that it is $\prediction(\Bpred(\cdot)) = \argmax_{y \in \Yc} p(y|x)$ were the same element $y$ is selected for all equivalent $x$). $\prediction(\Bpred(\cdot))$ is thus an invariant labeling $\labelingk{|\Yc|}$.
By \cref{lemma:kary_shatterability},  binary shatterability of $\p{Z | X}$ thus implies that there exists an $f \in \Q$ s.t. $\prediction(f(Z)) \aseq{} \prediction(\Bpred(X))$.
For all invariant tasks we thus have $\Risk{M(X)}{Z} = \RiskQ{M(X)}{X}{\U} = 0$ so $\p{Z|X} \in \dP{} $ as desired. 
\end{proof}

As seen in the proof, binary shatterability implies discriminativeness. 
We neverthless put emphasize the maximal invariant in \cref{appx:eqn:task_invariance}, because predictability of the maximinal invariant is more computationally efficient and, as shown in \toappx{}, implies discriminativeness with high likelihood when the dimension is large enough.
