# Supplementary material for: Improving Self-Supervised Learning by Characterizing Idealized Representations
Source: arXiv:2209.06235 source file (2022-12-12)
Supplement: Supplementary file 5 [file myths_sec.tex]

\clearpage
\newpage
