# Supplementary material for: Improving Self-Supervised Learning by Characterizing Idealized Representations
Source: arXiv:2209.06235 source file (2022-12-12)
Supplement: Supplementary file 6 [file checklist.tex]

%%%%%%%%%%%%%%%%%%%%%%%%%%%%%%%%%%%%%%%%%%%%%%%%%%%%%%%%%%%%


%%% BEGIN INSTRUCTIONS %%%


\begin{enumerate}


\item For all authors...
\begin{enumerate}
  \item Do the main claims made in the abstract and introduction accurately reflect the paper's contributions and scope?
   \answerYes{}
  \item Did you describe the limitations of your work?
    \answerYes{} in \cref{sec:discussion} expanded in \cref{sec:appx:discussion} .
  \item Did you discuss any potential negative societal impacts of your work?
    \answerNo{}.% in \cref{sec:appx:discussion}.
  \item Have you read the ethics review guidelines and ensured that your paper conforms to them?
     \answerYes{}
\end{enumerate}


\item If you are including theoretical results...
\begin{enumerate}
  \item Did you state the full set of assumptions of all theoretical results?
     \answerYes{} in  the paper the main paper we mention the important ones succintly, in \cref{sec:appx:prel:assumptions} we discuss each in detail.
        \item Did you include complete proofs of all theoretical results?
    \answerYes{} in \cref{sec:appx:proofs}.
\end{enumerate}


\item If you ran experiments...
\begin{enumerate}
  \item Did you include the code, data, and instructions needed to reproduce the main experimental results (either in the supplemental material or as a URL)?
   \answerYes{} all the code to reproduce our results can be found at \codeurl{}.
  \item Did you specify all the training details (e.g., data splits, hyperparameters, how they were chosen)?
     \answerYes{} in \cref{sec:appx:reproducability}.
        \item Did you report error bars (e.g., with respect to the random seed after running experiments multiple times)?
     \answerYes{} for the TinyImageNet table. We did not for ImageNet due to computational constraints.
        \item Did you include the total amount of compute and the type of resources used (e.g., type of GPUs, internal cluster, or cloud provider)?
    \answerNo{}.
\end{enumerate}


\item If you are using existing assets (e.g., code, data, models) or curating/releasing new assets...
\begin{enumerate}
  \item If your work uses existing assets, did you cite the creators?
   \answerYes{}.
  \item Did you mention the license of the assets?
  \answerNo{}.
  \item Did you include any new assets either in the supplemental material or as a URL?
    \answerNA{}.
  \item Did you discuss whether and how consent was obtained from people whose data you're using/curating?
    \answerNA{}.
  \item Did you discuss whether the data you are using/curating contains personally identifiable information or offensive content?
    \answerNo{}.
\end{enumerate}


\item If you used crowdsourcing or conducted research with human subjects...
\begin{enumerate}
  \item Did you include the full text of instructions given to participants and screenshots, if applicable?
    \answerNA{}.
  \item Did you describe any potential participant risks, with links to Institutional Review Board (IRB) approvals, if applicable?
    \answerNA{}.
  \item Did you include the estimated hourly wage paid to participants and the total amount spent on participant compensation?
  \answerNA{}.
\end{enumerate}


\end{enumerate}
