# Supplementary material for: Improving Self-Supervised Learning by Characterizing Idealized Representations
Source: arXiv:2209.06235 source file (2022-12-12)
Supplement: Supplementary file 7 [file results_old.tex]

\subsection{Approximations}

In this section we evaluate the effect of different approximations that we had to do for computational reasons.

\subsubsection{Effect of number of subtasks}

In \tocref{} we looked at the worst possible performance on \tofill{} randomly sampled binary tasks. This is an approximation of the real metric that we care (see \tocref{}), \ie, which is the worst possible invariant task.
The number of subpartitions, i.e., deterministic tasks to consider, is given by the Bell number $B_n$ \tocite{}. Solving that many tasks to find the the worst possible is computationally prohibitive. For example when $|\mathcal{M}|=10$ as is the case for MNIST, that would require taking the max over $B_n=115975$.
We thus make two assumptions:
\begin{itemize}
\item consider only binary tasks, as those are the ones that aggregate the most, and we conjecture that if we can solve all binary subpartions then we can solve all k-ary partitions; 
\item sample a few tasks, as considering all binary tasks for MNIST would require $S(|\mathcal{M}|,2)=511$ tasks which is still prohibitive. Here $S$ is the Stirling number of the second kind.
\end{itemize}
We now evaluate those approximations for MNIST. 
We do so for generative and contrastive ISSL models, both for standard and our variants.

\input{figures/mnist/effect_n_tasks}

\paragraph{The number of tasks has less effect on our ISSL.}
 \cref{fig:effect_n_tasks} shows that the number of tasks (number and type) has less on our ISSL (first two columns) compared to standard ISSL (last two columns).
Indeed, the performance gap between our ISSL and standard ISSL increases as the number of considered tasks increases from $4 \to 64$.
For contrastive ISSL: $0.3 \to 0.55$ pp.
For generative ISSL: $13 \to 17$ pp.
This suggests that using more tasks would only make our ISSL seem more compelling, and thus using fewer tasks due to computational reasons does not change the main take aways.

\paragraph{Binary tasks are better approximations.}
We see on  \cref{fig:effect_n_tasks}, as hypothesized, the hardest tasks seem to be binary tasks. Note that this is not the case for all binary tasks, which is why for standard generative model, binary tasks are have higher performance than ``all tasks''. For average case, it makes sense that binary tasks are easier simply because random prediction is already much better ($50\%$ against $10\%$ for all tasks).
This supports our choice of binary tasks throughout our paper.


\paragraph{32 tasks gives a good approximation.}
From  \cref{fig:effect_n_tasks}, we see that the accuracy decreases significantly and monotonically with the number of tasks.
Although more tasks continue decreasing the accuracy, $32$ generally seems to give decent approximations while being manageable computationally. This is why we use 32 tasks whenever we want good approximations of the worst case performance.
Otherwise we use 16 tasks throughout the paper.


\clearpage
\newpage

\subsection{Testing the theory}
\label{appx:results:testing_theory}

\subsubsection{Controlled experiments}
\label{appx:results:controlled}

In the main paper we have evaluated the theory in well controlled experiments.
Here we provide all the results that have only been hinted towards in the main text due to space limitation.


\input{figures/controlled/regularization}

\paragraph{Effect of regularization on dimensionality and sample efficiency?}
As discussed in the main text, the minimal achievable dimensionality and sample efficiency can only be achieved if equivalent examples $x \sim x^+$ get mapped to the same representations $z$, but the ISSL objective only ensures that non-equivalent examples $x \not\sim x^-$  are mapped to different representations $z,z^-$.
To achieve the former we can add an additional regularizer (see \tocref{}).
 \Cref{fig:regularizers} shows indeed that adding a regularizer is necessary to achieve the optimal dimension $d(\Q)=10$ (\cref{fig:reg_dim}) and sample efficiency $\rS{}$ (\cref{fig:reg_samples}).
Furthermore, we see that in both cases the need for a regularizer decreases when training for longer.
This suggests that training for longer can have the desired implicit regularization effect, which could explain why long training times are so important in practical ISSL \cite{}.
We hypothesize that the implicit regularzation effect comes from the noise in SGD which essentially minimizes some form of $\MI{Z}{X}$ \cite{shwar}. %Opening black box


\input{tables/controlled/appcs/exact_losses}
\input{tables/controlled/appcs/exact_losses_test}
\paragraph{Effect of using the wrong loss?}
In \tocref{} we prove that any \tofill{} loss can be used during ISSL to achieve optimal representations, and surprisingly this is independent of the choice of downstream losses.
\Cref{tab:exact_losses} empirically supports our claim by showing that any of MSE / hinge / log loss used during ISSL can learn optimal representations.
Furthermore, we see that performance w.r.t. specific downstream loss (MSE / hinge / 0-1/ log loss) is uncorrelated with the loss used during ISSL.
Note that our theoretical results say nothing about when ISSL is not perfect (e.g. approximate optimizers and only access to samples) in which case the choice of loss is actually important.
\Cref{tab:exact_losses_test} shows that even when ISSL is not optimal (using access to samples) the choice of loss for ISSL and prediction still seem uncorrelated.



\input{tables/controlled/appcs/exact_permMx}

\paragraph{Do augmentations need to retain labels?}
It is often said \tocite{} that data augmentations should not change the label of the underlying example. 
We have seen in \tocref{} that actually this is not a necessary requirement, the necessary and sufficient requirement essentially says that if the Bayes predictor of the augmentation is the same then so should the labels the examples, i.e., $\bayesA{\A \cond X}(x) = \bayesA{\A \cond X}(x')  \implies x \sim x'$.
In practice this means that input examples (e.g. an image of an ``8'') can be augmented to output examples that would generally have different labels (e.g. an image of a ``9''), as long as this is the case for all equivalent examples (e.g. all ``8'' get augmented to ``9'').
We show that this indeed the case in \cref{tab:exact_permMX} by comparing exact augmentations to augmentations to permuted $M(X)$ in the case of exact (``train'') and samples estimates (``test'') ISSL.
When using exact ISSL, this should be quite intuitive as this simply corresponds to permuting the weight matrix of the last linear predictor.
Perhaps more suprisingly we show in \cref{tab:cntr_permMX} that the same holds when using contrastive learning and finite samples, which disproves the typical explanation of contrastive learning as ``bringing augmented and non-augmented examples closer together''.


\subsubsection{Practical setting}
\label{appx:results:practical}

In the following we show that the trends we saw in the main controlled experiments (\cref{sec:controlled_exp}) in the typical practical setting where we use approximate ISSL objectives (here contrastive) and do not assume access to the underlying unlabelled distribution $p(X)$.
Although our theory does not cover this setting we show that generally the same trend hold, which suggests that our theory provides the right intuition in practical settings and can likely be generalized to cover those such case of practical/approximate ISSL.
To minimize computation we run only the core experiments.


\input{figures/cntr_controlled/aug}

\paragraph{Effect of augmentations on required dimensionality?}
In \cref{fig:aug_dim} we have seen that, as predicted by theory,  using any sufficient augmentation one can achieve perfect performance for a certain dimensionality of $Z$.
Importantly, this required dimensionality decreases as the augmentation becomes coarser.
\Cref{fig:cntr_aug_dim} shows exactly the same trend with best performance achieved from a dimensionality of $d(\Q)=10$ when using optimal augmentations.


\paragraph{Effect of augmentations on sample efficiency?}
In \cref{fig:aug_sample} we have seen that, as predicted by theory, using any sufficient augmentation one can achieve perfect performance when downstream predictors are trained on enough samples.
Importantly, this required number of samples decreases as the augmentation becomes coarser.
\Cref{fig:cntr_aug_sample} shows exactly the same trend with best performance achieved from a dimensionality of $\op{S_{\scriptscriptstyle \Q^-}}{\tasksinv{}|Z}=10$ when using optimal augmentations.



\input{figures/cntr_controlled/func_family}

\paragraph{Effect of using the wrong $\Q$?}
\tofill{}
\ydnote{
This is the only currently bad results, not sure what do here}



\paragraph{Effect of $\Q$ on the dimensionality?}
In \cref{fig:V_dim} we have seen that, as predicted by theory, more complex (in terms of VC dimension) downstream predictors require a smaller dimensionality of $Z$ to achieve the highest possible predictions.
\Cref{fig:V_dim} shows that the same trends holds for for approximate contrastive learning.
Just as the theory says, the optimal prediction seems to be achieved when the VC dimension is $|\mathcal{X} / \sim|-1$ which for linear predictor is $9$.



\input{tables/controlled/appcs/cntr_permMx}

\paragraph{Augmentations do not need to retain labels}
In \cref{tab:exact_permMX} we have seen that, as predicted by theory, the augmentation can change the underlying labels as long as the change is predictable.
\cref{tab:cntr_permMX} shows the same essentially holds when considering the practical setting of contrastive (i.e. approximate) ISSL and evaluating on unseen test points.





\subsubsection{Approximate ISSL objectives: generative, contrastive, self-distillation}
\label{appx:results:approx_ISSL}

In the last two subsection we have shown experiment that support our theory in
\begin{inlinelist}
\item settings that are as close as possible to our assumptions, i.e., exact ISSL with $p(X)$;
\item practical settings with contrastive learning and finite sample estimation.
\end{inlinelist}
In the following we show that the same trend essentially hold for other approximate ISSL, specifically, generative and self-distillation models.
As all experiment require hundreds of runs, we consider focus on the small MNIST dataset which is sufficient to show that the same trends hold and avoids unnecessary computation.
%Importantly, this is only about the approximate ISSL object, but we still focus on the the case where the unlabelled distribution $p(X)$ is accessible, we consider finite sample setting in the next section.

% All results are summarized in \cref{tab:appcs:mnist}.
% The first row ``supervised'' shows the performance of a supervised model, while the next four blocks ``exact'', ``generative'', ``contrastive'', ``self-distillation'' refer to the objective used of ISSL (see \tocref{}).
% In each block ``Standard'' corresponds to the standard objective for that type while ``ours'' refer to our proposed small modifications.
% All rows use standard augmentations besides the ``opt. aug.'' rows which use optimal augmentations.
% ``$\Q$'' and ``$\Q^+$'' refer to the predictive family of both the predictor and ISSL.
% By default no regularization is used besides in the rows ``reg.''.
% For columns $\rS{}$ is the estimated sample efficiency, $d(\Q)$ is the estimated minimal required dimension, 
% ``$\RiskA{M(X)}{Z}$  train'' shows the training performance, \ie, says whether the information is decodable and assumes the unlabeled $p(X)$ is seen during training. 
% ``$\RiskA{M(X)}{Z}$'' is the same but on the test set, \ie, the practical objective people care about.
% ``$\sup_Y \RiskA{Y}{Z}$'' shows the test performance on the worst invariant task, \ie, coarsening of the MNIST task such as whether the digit is odd or even.
% ``100 labels'' shows the test performance $\RiskA{M(X)}{Z}$ but when only a few labels are seen ,\ie, essentially semi-supervised learning.
% ``$\times$'' means that we did not find a good estimate of the desired values.

% \input{tables/controlled/appcs/mnist}

% \ydnote{might just drop all the columns besides d and s estimate. I'm not sure what the rest gives as information.
% Might even just keep them for opt aug and non opt aug.
% }



\input{tables/controlled/appcs/mnist_samples}



\paragraph{Does approximating the ISSL objective change the required sample efficiency $\rS{}$?}
From \tocref{} we know that the required sample efficiency should be $\rS{}=10$ when using optimal augmentations.
We have seen in \cref{fig:aug_sample} and \cref{fig:cntr_aug_sample} that this value is recovered both in the controlled (exact ISSL) and practical (contrastive) setting for CIFAR10.
\Cref{tab:appcs:mnist} shows that the same $\rS{}=10$ essentially holds for MNIST and self-distillation and generative approximations of the ISSL objective.
Note that for self-distillation we actually get $\rS{}=100$, we believe that this is due to practical optimization issues.
Importantly when using non standard augmentations we get larger $\rS{}$ as suggested in \cref{fig:aug_sample}.


\input{tables/controlled/appcs/mnist_dim}

\paragraph{Does approximating the ISSL objective change the required dimensionality $d(\Q)$?}
From \tocref{} we know that the required dimensionality should be $d(\Q)=9$ when using optimal augmentations.
\ydnote{actually it's annoying because in reality the required dimensionality should be 9 but we only tested the closest 9}
We have seen in \cref{fig:aug_dim} and \cref{fig:cntr_aug_dim} that this value is recovered both in the controlled (exact ISSL) and practical (contrastive) setting for CIFAR10.
\Cref{tab:appcs:mnist} shows that the same $d(\Q)=10$ essentially holds for MNIST and self-distillation and generative approximations of the ISSL objective.
Note that for self-distillation we actually get $d(\Q)=16$ which is the next dimension we tested, we believe that this is due to practical optimization issues.
Importantly when using non standard augmentations we get larger $d(\Q)$ as suggested in \cref{fig:aug_dim}.


\input{tables/controlled/appcs/mnist}



\clearpage
\newpage

\subsection{Realistic}
\label{appx:results:realistic}

\input{tables/realistic/appcs}
